# Supplementary material for: Online Combinatorial Linear Optimization via a Frank-Wolfe-based Metarounding Algorithm
Source: arXiv:2310.12629 source file (2023-11-19)
Supplement: Supplementary file 1 [file appendix.tex]

\begin{lemma}
    The Lagrange dual problem of (\ref{eq:main-primal}) is
    \begin{align}
        \label{eq:main-dual}
        \max_{\gamma, \bm{\ell}} \; \gamma
        \qquad
        \text{s.t.} \quad
        &
        \bm{\ell} \cdot \bm{c} \geq \gamma,
        \quad \forall \bm{c} \in \combset, \\
        \nonumber
        & \bm{\ell} \cdot \bm{x} = 1, \\
        \nonumber
        & \bm{\ell} \geq \bm{0}.
    \end{align}
\end{lemma}
\begin{proof}
    Let $
        \bm{\ell} \in \real^{n}_{+},
        \gamma \in \real,
        \bm{\mu} \in \real^{\combset}_{+}
    $ be the Lagrange variables.
    We can construct the Lagrangian %
    $L(\beta, \bm{\lambda}; \bm{\ell}, \gamma, \bm{\mu})$ as
    \begin{align*}
        L(\beta, \bm{\lambda}; \bm{\ell}, \gamma, \bm{\mu})
        =
        \beta
        + \sum_{i=1}^{n} \ell_{i} \left(
            \sum_{\bm{c} \in \combset} \lambda_c c_{i} - \beta x_{i}
        \right)
        + \gamma \left(
            1 - \sum_{\bm{c} \in \combset} \lambda_{\bm{c}}
        \right)
        - \sum_{\bm{c} \in \combset} \mu_{\bm{c}} \lambda_{\bm{c}}.
    \end{align*}
    Differentiating $L$ w.r.t. the primal variables
    $\beta, \lambda_{\bm{c}}$ and set them as $0$,
    we have
    \begin{alignat*}{2}
        \frac{\partial}{\partial \beta} L
        = \; & 1 - \bm{\ell} \cdot \bm{x} = 0
        % = & 1 - \sum_{i=1}^{n} \ell_{i} x_{i} = 0
          & \implies \quad & \bm{\ell} \cdot \bm{x} = 1, \\
        \frac{\partial}{\partial \lambda_{\bm{c}}} L
        = \; & \bm{\ell} \cdot \bm{c} - \gamma - \mu_{\bm{c}} = 0
        % = & \sum_{i=1}^n \ell_i c_i - \gamma - \mu_{\bm{c}} = 0
        \quad
          & \implies \quad & \bm{\ell} \cdot \bm{c} \geq \gamma.
    \end{alignat*}
    Plugging these conditions to $L$, we get the dual problem.
    \qed
\end{proof}
